# Supplementary material for: Spin-density wave of ferrimagnetic building blocks masking the ferromagnetic quantum-critical point in NbFe2
Source: arXiv:2601.00101 ancillary file (2026-11-06)
Supplement: Supplementary file 1 [file NbFe2_diffraction_supplement_v1.pdf]

# Spin-density wave of ferrimagnetic building blocks masking a ferromagnetic quantum-critical point in $NbFe_2$ - supplemental information

T. Poulis,[1] G. Mani,[1] J. Sturt,[1] W. J. Duncan,[1] H. Thoma,[2] V. Hutanu,[2] B. Ouladdiaf,[3] I. Kibalin,[3] M. H. Lemee,[3] P. Manuel,[4] A. Neubauer,[5] C. Pfleiderer,[5] F. M. Grosche,[6] and P. G. Niklowitz[1]

[1]*Department of Physics, Royal Holloway, University of London, Egham TW20 0EX, United Kingdom*
[2]*Institute of Crystallography, RWTH University, Aachen 52066, Germany*
[3]*Institute Laue Langevin, Grenoble 38042 - CS 20156, France*
[4]*Isis Neutron Source, STFC Rutherford Appleton Laboratory, Didcot OX11 0QX, United Kingdom*
[5]*Physik Department E21, Technische Universität München, 85748 Garching, Germany*
[6]*Cavendish Laboratory, University of Cambridge, Cambridge CB3 0HE, United Kingdom*

(Dated: December 31, 2025)

## NUMERICAL SNP ANALYSIS

Data analysis employed the software FileScanner [1] that accounts for the decaying polarization of the analyser and polariser. This software draws on all 36 polarization channels, with each intensity representing a combination of various scattering factors as shown in Table I. Scattering factors are optimised with least-squares fitting.

TABLE I. SNP cross sections obtained from the Blume-Maleev equations [2]; each $\sigma_{ij}$ term on the left is equal to the sum of the terms on the right.

| $\sigma_{ij}$ | Nuclear | Magnetic | Chiral Magnetic | Nuclear-Magnetic Interference |
|---|---|---|---|---|
| $xx$ | $NN^*$ | | | |
| $x\overline{x}$ | | $M_\perp M_\perp^*$ | $-i(M_\perp \times M_\perp^*)$ | |
| $\overline{x}x$ | | $M_\perp M_\perp^*$ | $+i(M_\perp \times M_\perp^*)$ | |
| $\overline{xx}$ | $NN^*$ | | | |
| $yy$ | $NN^*$ | $M_y M_y^*$ | | $+2Re[NM_y^*]$ |
| $y\overline{y}$ | | $M_z M_z^*$ | | |
| $\overline{y}y$ | | $M_z M_z^*$ | | |
| $\overline{yy}$ | $NN^*$ | $M_y M_y^*$ | | $-2Re[NM_y^*]$ |
| $zz$ | $NN^*$ | $M_z M_z^*$ | | $+2Re[NM_z^*]$ |
| $z\overline{z}$ | | $M_y M_y^*$ | | |
| $\overline{z}z$ | | $M_y M_y^*$ | | |
| $\overline{zz}$ | $NN^*$ | $M_z M_z^*$ | | $-2Re[NM_z^*]$ |
| $xy = y\overline{x}$ | $NN^*/2$ | $M_\perp M_\perp^*/2$ | $-i(M_\perp \times M_\perp^*)/2$ | $+Re[NM_y^*] + Im[NM_z^*]$ |
| $x\overline{y} = \overline{yx}$ | $NN^*/2$ | $M_\perp M_\perp^*/2$ | $-i(M_\perp \times M_\perp^*)/2$ | $-Re[NM_y^*] - Im[NM_z^*]$ |
| $\overline{x}y = yx$ | $NN^*/2$ | $M_\perp M_\perp^*/2$ | $+i(M_\perp \times M_\perp^*)/2$ | $+Re[NM_y^*] - Im[NM_z^*]$ |
| $\overline{xy} = \overline{y}x$ | $NN^*/2$ | $M_\perp M_\perp^*/2$ | $+i(M_\perp \times M_\perp^*)/2$ | $-Re[NM_y^*] + Im[NM_z^*]$ |
| $xz = z\overline{x}$ | $NN^*/2$ | $M_\perp M_\perp^*/2$ | $-i(M_\perp \times M_\perp^*)/2$ | $+Re[NM_z^*] - Im[NM_y^*]$ |
| $x\overline{z} = \overline{zx}$ | $NN^*/2$ | $M_\perp M_\perp^*/2$ | $-i(M_\perp \times M_\perp^*)/2$ | $-Re[NM_z^*] + Im[NM_y^*]$ |
| $\overline{x}z = zx$ | $NN^*/2$ | $M_\perp M_\perp^*/2$ | $+i(M_\perp \times M_\perp^*)/2$ | $+Re[NM_z^*] + Im[NM_y^*]$ |
| $\overline{xz} = \overline{z}x$ | $NN^*/2$ | $M_\perp M_\perp^*/2$ | $+i(M_\perp \times M_\perp^*)/2$ | $-Re[NM_z^*] - Im[NM_y^*]$ |
| $yz = z\overline{y}$ | $NN^*/2$ | $M_\perp M_\perp^*/2 + Re[M_y M_z^*]$ | | $+Re[NM_y^*] + Re[NM_z^*]$ |
| $y\overline{z} = \overline{zy}$ | $NN^*/2$ | $M_\perp M_\perp^*/2 - Re[M_y M_z^*]$ | | $+Re[NM_y^*] - Re[NM_z^*]$ |
| $\overline{y}z = zy$ | $NN^*/2$ | $M_\perp M_\perp^*/2 - Re[M_y M_z^*]$ | | $-Re[NM_y^*] + Re[NM_z^*]$ |
| $\overline{yz} = \overline{z}y$ | $NN^*/2$ | $M_\perp M_\perp^*/2 + Re[M_y M_z^*]$ | | $-Re[NM_y^*] - Re[NM_z^*]$ |

## ANALYTICAL SNP ANALYSIS

Table II presents the equations utilized for calculating the scattering factors via the analytical method. The indices $i = (1, 2, 3)$ denote different calculations of the same scattering factor, with each corresponding to a distinct set of intensities. For instance, $NN_1$, $NN_2$, and $NN_3$ all relate to the nuclear scattering factor $NN$, but are derived from separate combinations of SNP cross sections as listed in Table II.

In Table III the results of the analytical determination of scattering factors from SNP cross sections are given for both SDW Bragg peak positions investigated.

TABLE III. Scattering Factors obtained analytically from SNP scattering cross sections.

| **Scattering Factors** | **Q = (2 -2 -1.1)** | **Q = (2 -2 -3.1)** |
|---|---|---|
| $NN_1^*$ | $0.006 \pm 0.005$ | $0.024 \pm 0.023$ |
| $NN_2^*$ | $0.128 \pm 0.030$ | $0.001 \pm 0.001$ |
| $NN_3^*$ | $0.083 \pm 0.027$ | $0.001 \pm 0.0182$ |
| $M_y M_{y\,1}^*$ | $6.902 \pm 0.260$ | $2.240 \pm 0.156$ |
| $M_y M_{y\,2}^*$ | $7.586 \pm 0.395$ | $2.528 \pm 0.147$ |
| $M_z M_{z\,1}^*$ | $0.006 \pm 0.006$ | $0.033 \pm 0.034$ |
| $M_z M_{z\,2}^*$ | $0.022 \pm 0.005$ | $0.012 \pm 0.009$ |
| $i(M_\perp \times M_\perp^*)_1$ | $0.000 \pm 0.000$ | $-0.102 \pm 0.160$ |
| $i(M_\perp \times M_\perp^*)_2$ | $-0.550 \pm 0.129$ | $-0.160 \pm 0.069$ |
| $i(M_\perp \times M_\perp^*)_3$ | $-0.012 \pm 0.031$ | $0.112 \pm 0.180$ |
| $Re(M_y M_z^*)$ | $-0.127 \pm 0.170$ | $-0.159 \pm 0.069$ |
| $Re(NM_y^*)_1$ | $0.003 \pm 0.293$ | $0.000 \pm 0.137$ |
| $Re(NM_y^*)_2$ | $0.708 \pm 0.151$ | $-0.000 \pm 0.069$ |
| $Re(NM_y^*)_3$ | $0.132 \pm 0.034$ | $0.000 \pm 0.120$ |
| $Re(NM_z^*)_1$ | $-0.053 \pm 0.068$ | $-0.005 \pm 0.032$ |
| $Re(NM_z^*)_2$ | $-0.002 \pm 0.015$ | $0.000 \pm 0.006$ |
| $Re(NM_z^*)_3$ | $0.001 \pm 0.000$ | $0.001 \pm 0.002$ |
| $Im(NM_y^*)$ | $0.000 \pm 0.000$ | $0.090 \pm 0.199$ |
| $Im(NM_z^*)$ | $0.000 \pm 0.000$ | $-0.013 \pm 0.036$ |

TABLE II. Analytical expressions of scattering factors in terms of SNP cross sections.

$$
\begin{aligned}
NN_1^* &= \frac{(\sigma_{zz}+\sigma_{\overline{zz}}-\sigma_{y\overline{y}}-\sigma_{\overline{y}y})}{2}\\
NN_2^* &= \frac{(\sigma_{yy}+\sigma_{\overline{yy}}-\sigma_{z\overline{z}}-\sigma_{\overline{z}z})}{2}\\
NN_3^* &= \frac{(\sigma_{xx}+\sigma_{\overline{xx}})}{2}\\
M_yM_y^*{}_1 &= \frac{(\sigma_{z\overline{z}}+\sigma_{\overline{z}z})}{2}\\
M_yM_y^*{}_2 &= \frac{(\sigma_{x\overline{x}}+\sigma_{\overline{x}x}-\sigma_{\overline{y}y}-\sigma_{y\overline{y}})}{2}\\
M_zM_z^*{}_1 &= \frac{(\sigma_{y\overline{y}}+\sigma_{\overline{y}y})}{2}\\
M_zM_z^*{}_2 &= \frac{(\sigma_{x\overline{x}}+\sigma_{\overline{x}x}-\sigma_{\overline{z}z}-\sigma_{z\overline{z}})}{2}\\
i(M_\perp\times M_\perp^*)_1 &= \frac{(\sigma_{\overline{x}y}+\sigma_{\overline{xy}}-\sigma_{xy}-\sigma_{x\overline{y}})}{4}\\
i(M_\perp\times M_\perp^*)_2 &= \frac{(\sigma_{\overline{x}x}-\sigma_{x\overline{x}})}{2}\\
i(M_\perp\times M_\perp^*)_3 &= \frac{(\sigma_{\overline{x}z}+\sigma_{\overline{xz}}-\sigma_{xz}-\sigma_{x\overline{z}})}{2}\\
Re(NM_y^*)_1 &= \frac{(\sigma_{yy}-\sigma_{\overline{yy}})}{4}\\
Re(NM_y^*)_2 &= \frac{(\sigma_{xy}-\sigma_{\overline{xy}}+\sigma_{\overline{x}y}-\sigma_{x\overline{y}})}{4}\\
Re(NM_y^*)_3 &= \frac{(\sigma_{yz}-\sigma_{\overline{yz}}+\sigma_{y\overline{z}}-\sigma_{\overline{y}z})}{4}\\
Re(NM_z^*)_1 &= \frac{(\sigma_{zz}-\sigma_{\overline{zz}})}{4}\\
Re(NM_z^*)_2 &= \frac{(\sigma_{xz}-\sigma_{\overline{xz}}+\sigma_{\overline{x}z}-\sigma_{x\overline{z}})}{4}\\
Re(NM_z^*)_3 &= \frac{(\sigma_{yz}-\sigma_{\overline{yz}}+\sigma_{\overline{y}z}-\sigma_{y\overline{z}})}{4}\\
Im(NM_y^*) &= \frac{(\sigma_{x\overline{z}}+\sigma_{\overline{x}z}-\sigma_{xz}-\sigma_{\overline{xz}})}{4}\\
Im(NM_z^*) &= \frac{(\sigma_{xy}+\sigma_{\overline{xy}}-\sigma_{x\overline{y}}-\sigma_{\overline{x}y})}{4}\\
Re(M_yM_z^*) &= \frac{(\sigma_{yz}+\sigma_{\overline{yz}}-\sigma_{\overline{y}z}-\sigma_{y\overline{z}})}{4}
\end{aligned}
$$

## FITTING PEAKS FROM D10+ WITH POSITION-SENSITIVE DETECTOR

Nuclear Bragg peaks at 20 K were collated at D10+ without an analyser and with using a position-sensitive detector (PSD). The Bragg peaks have been fitted with a modified Gaussian function.

While $Q$ peaks could be fitted well with a combined constant-background and simple-Gaussian model, higher-$Q$ peak shapes are more complex due to increased instrumental resolution effects and are better fitted by replacing the simple-Gaussian part with the phenomenological modified-Gaussian model

$$A \cdot e^{-(x-B)/C(\theta))^2} \tag{1}$$

with

$$C(\theta)^2 = U \cdot tan(\theta)^2 + W + \frac{P}{cos(\theta)^2}\ . \tag{2}$$

To calculate peak-intensity uncertainties residual analysis has been used instead of standard error propagation due to the large number of fitted parameters.

In Fig. 1 and Fig. 2 fits of $\vec{Q}$ =(1 0 0) and $\vec{Q}$ =(0 0 6) are given as low- and high-$Q$ examples, respectively.

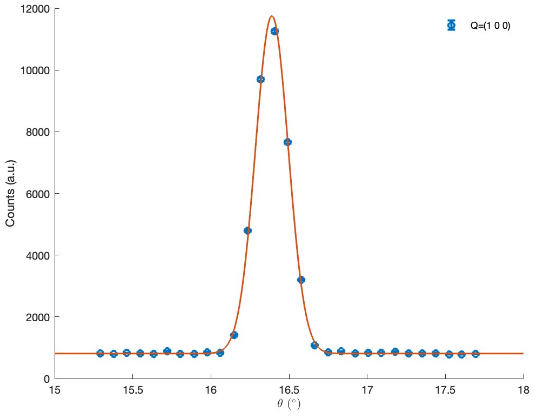


FIG. 1. Modified Gaussian fit of the $\vec{Q} = (100)$ reflection at $T = 20\,\mathrm{K}$ obtained at D10+.

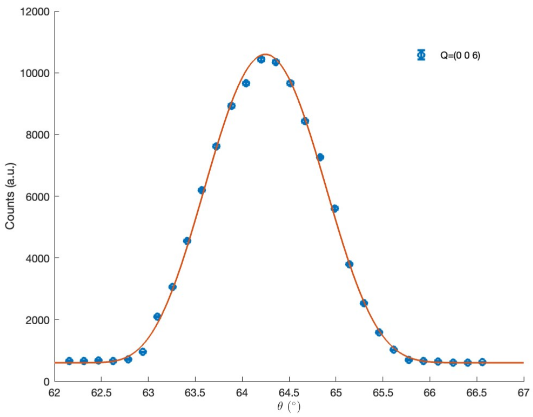


FIG. 2. Modified Gaussian fit of the $\vec{Q} = (006)$ reflection at $T = 20\,\mathrm{K}$ obtained at D10+.

## FITTING PEAKS FROM D10+ WITH SINGLE-COUNTER DETECTOR

Nuclear and magnetic Bragg peaks at 4 K were collated at D10+ with a set-up including an analyser, aperture and single-counter detector. The analyser reduces the inelastic background sufficiently to well resolve the low-moment magnetic Bragg peaks. However, in this set up, during rocking scans, tails of Bragg peaks are cut off. As a result, simple Gaussians fit the resulting peaks well, but only the amplitudes can be extracted from those fits with high certainty. Fig. 3 shows a magnetic $\vec{Q}$ position with no peak. Fig. 4 and Fig. 5 show examples of magnetic peaks at low- and high-$Q$ positions, respectively.

To arrive at realistic peak widths the Caglioti formula

$$c = \sqrt{c_0^2 + u \cdot \tan(\theta) + w \cdot \tan^2(\theta)}$$

has been used. $c$ is the Gaussian peak width and fit

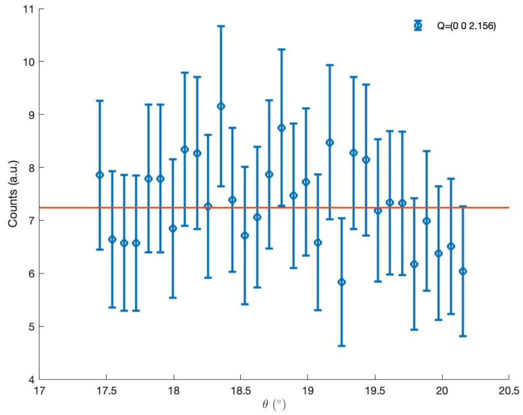


FIG. 3. Magnetic position $\vec{Q} = (0\ 0\ 2.156)$ with no peak detected at $T = 4\,\mathrm{K}$. Data measured at D10+

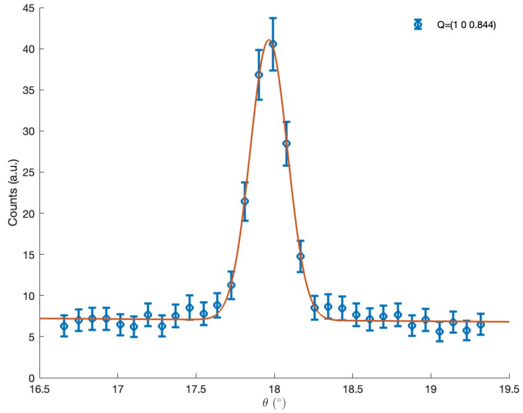


FIG. 4. Gaussian fit of $\vec{Q} = (1\ 0\ 0.844)$ magnetic peak at $T = 4\,\mathrm{K}$ obtained at D10+.

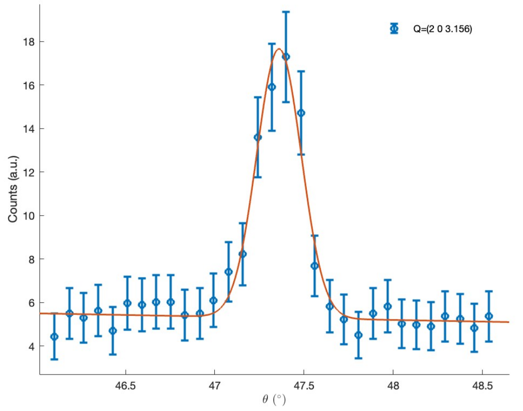


FIG. 5. Gaussian fit of $\vec{Q} = (2\ 0\ 3.156)$ magnetic peak at $T = 4\,\mathrm{K}$ obtained at D10+.

parameters $c_0$, $u$ and $w$ are dependent on the monochromator and sample mosaicity and beam divergence. $w > 0$ so increased peak broadening is expected towards larger $Q$. For D10+ in parallel position $u < 0$ is required. Fit-parameter values have been obtained by application of the Caglioti formula to the nuclear Bragg peaks at $20\,\mathrm{K}$ (Fig. 6) that had been measured with a PSD. This method corrected the magnetic intensities to their non-clipped values.

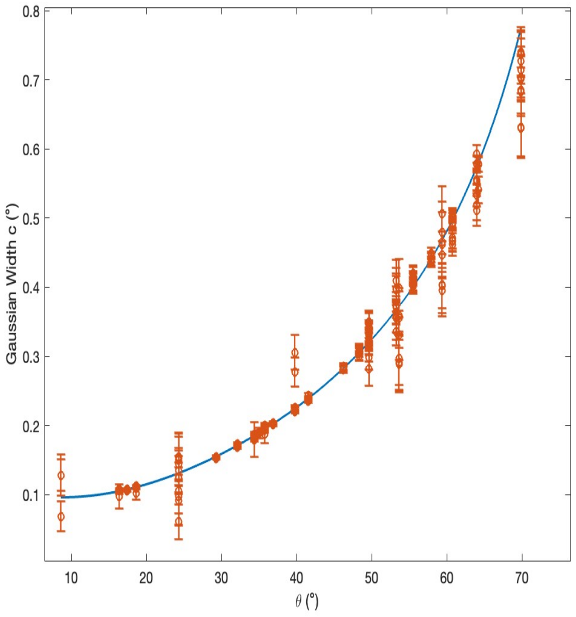


FIG. 6. Scattering angle dependence of the nuclear peak widths at $20\,\mathrm{K}$ measured with a PSD detector. The data is fitted with the Caglioti formula: $c = \sqrt{c_0^2 + u \cdot \tan(\theta) + w \cdot \tan^2(\theta)}$, with the fit parameters $c_0 = 0.107(2)$, $w = 0.089(2)$, and $u = -0.027(1)$.

## FITTING PEAKS FROM WISH

A few magnetic peaks have also been measured with time-of-flight (TOF) spectrometer WISH at ISIS in order to confirm the scale of the proposed moments. Using the software Mantid [3] peak shapes have been fitted with a convolution of back-to-back exponentials with a Gaussian function: [4]

$$c(x) = I \cdot \frac{AB}{2 \cdot (A+B)} \cdot$$

$$\left[ \exp\left( \frac{A\left(AS^2 + 2(x - X_0)^2\right)}{2} \right) \mathrm{erfc}\left( \frac{AS^2 + (x - X_0)}{S \cdot \sqrt{2}} \right) + \right.$$

$$\exp\left(\frac{B\left(BS^2-2(x-X_0)\right)}{2}\right)\mathrm{erfc}\left(\frac{(BS^2-(x-X_0))}{S\cdot\sqrt{2}}\right)\Bigg]$$

where $I$ is the integrated peak intensity, $A$ and $B$ represent the absolute values of the exponential rise and decay constants modeling the TOF neutron pulse coming from the moderator, $S$ represents the standard deviation of the Gaussian and $X_0$ is the peak location, located at an $x$ below the peak maximum. Examples of fitted nuclear and magnetic peaks are shown in Fig. 7 and Fig. 8.

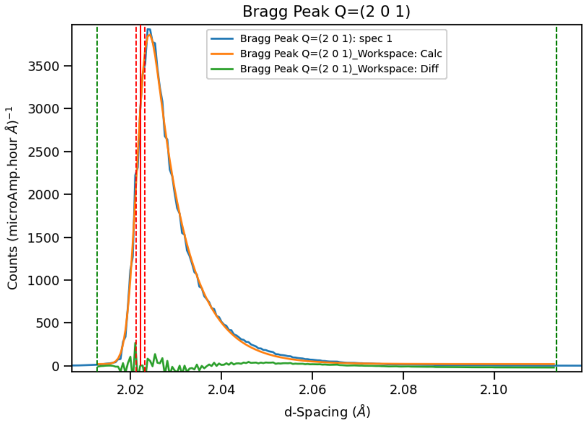


FIG. 7. Fitted nuclear peak $\vec{Q}$ = (2 0 1) at T = 1 K obtained at WISH. The fit model is described in the text.

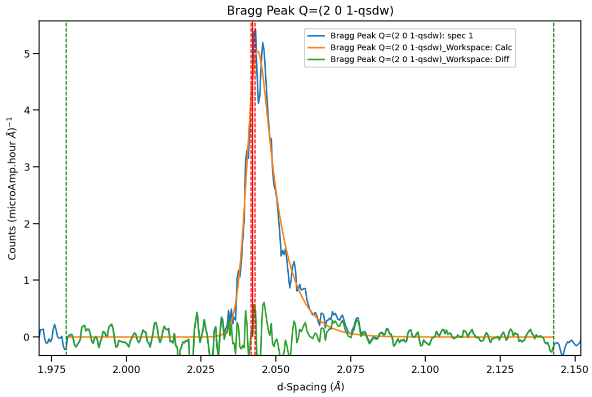


FIG. 8. Fitted magnetic peak $\vec{Q}$ = (2 0 0.844) at T = 1 K obtained at WISH. The fit model is described in the text.

## TECHNICAL DETAILS OF THE D10+ EXPERIMENT

The $T$ dependence of neutron diffraction of the SDW peak Q=(0 -2 0.844) revealed a transition temperature from SDW to PM of $T_{\mathrm{N}}$=15.3 K, close to the value of $T_{\mathrm{N}}$=14.8 K, reported for this sample at a previous neutron experiment [5].

To verify the crystal structure at 20 K, D10+ was used with a two-dimensional (2D) microstrip position-sensitive detector (PSD).

## NUCLEAR REFINEMENT IN THE PARAMAGNETIC STATE

At 20 K, 302 nuclear peaks have been measured that group into 31 symmetrically independent groups of reflections; 6 symmetrically forbidden groups that show peak absences have been removed from crystal symmetry considerations (e.g. $\vec{Q}$ = (0 0 1)). Additionally, the $\vec{Q}$ = (1 1 4) intensity appeared to be an experimental outlier and was removed from the final refinement. Data has been normalized to the monitor count. The Lorentz factor correction $\frac{1}{sin(2\theta)}$ for an $\omega$ scan in the equatorial plane has been used [6]. The average peak intensity was 45900 counts.

After calculating the lattice parameters from the centers of the peaks, Rietveld refinement was conducted using FullProf. First, the scale and the isotropic extinction parameters were refined, followed by the atomic positions. After that, the atomic occupancies were refined but were found to be very similar to the stoichiometric values as expected for a minimal replacement of 0.3% Nb by Fe. Therefore, stoichiometric values were fixed for the refinement of other parameters. The possibility of anti-site occupancy was also explored but did not improve the refinement as well as refinement of the isotropic temperature factor $b_{iso}$.

A comparison of measured Bragg peak intensities and calculated values based on Rietveld refinement is shown in Fig. 9. Associated refined parameters are listed in Table IV. Lattice parameters agreed with published values [7] and there is good agreement in general between obtained diffraction data and refinement based on the published [7] structure. Slight differences might be related to only few key parameters having been refined, and to indications of other crystallites in the sample seen during Laue Diffraction, which might have led to slight differences between the measured intensities of some symmetrically equivalent peaks. Data of the same sample at WISH with its high $Q$ resolution shows a small peak next to the main one at $\vec{Q}$ =(0 0 4) with an intensity that matches the difference between calculated intensity and the intensity observed at D10+.

## NUCLEAR REFINEMENT IN THE SDW STATE

To verify the crystal structure at 4 K, 150 nuclear peaks were measured. We corrected the intensities for the single-counter-detector influence on the measured peak widths (as described above) and for saturation due to the single detector's lower saturation threshold (approx-

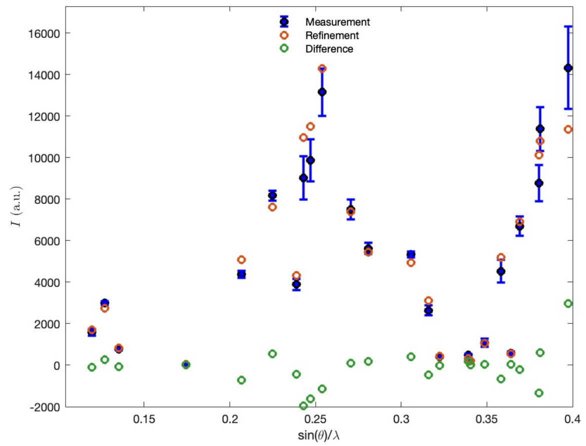


FIG. 9. Crystal structure of $NbFe_2$ at 20 K: measured and calculated Bragg peak intensities.

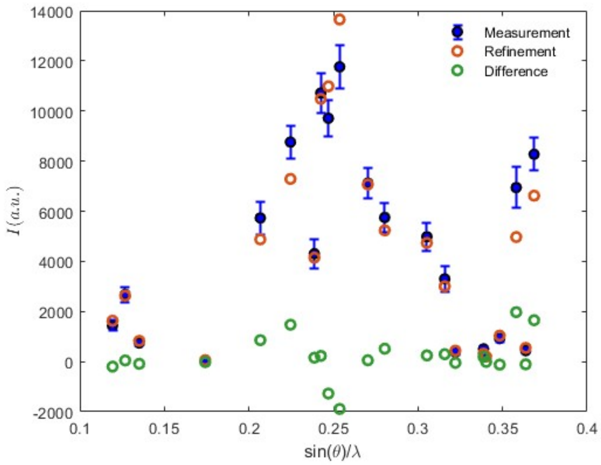


FIG. 10. Crystal structure of $NbFe_2$ at 4 K: measured and calculated Bragg peak intensities.

TABLE IV. Refined parameters of crystal structure at 20 K.

| Atom Site | x | y | z |
|---|---|---|---|
| Fe2a | 0 | 0 | 0 |
| Fe6h | 0.82960 | 0.17040 | 0.25000 |
| Nb | 0.33333 | 0.66667 | 0.06675 |
| Scale | 144.6 | | |
| Extinction | 6.151 | | |
| $b_{iso}$ | 0.0000 | | |
| $a(Å)$ | 4.833000 | | |
| $b(Å)$ | 4.833000 | | |
| $c(Å)$ | 7.874002 | | |
| $RF_2$ | 11.39 | | |
| $RF_2w$ | 10.18 | | |
| $RF$ | 5.479 | | |
| $\chi_2$ | 3.241 | | |

TABLE V. Refined parameters of crystal structure at 4 K.

| Atom Site | x | y | z |
|---|---|---|---|
| Fe2a | 0 | 0 | 0 |
| Fe6h | 0.82960 | 0.17040 | 0.25000 |
| Nb | 0.33333 | 0.66667 | 0.06675 |
| Scale | 144.6 | | |
| Extinction | 6.151 | | |
| $b_{iso}$ | 0.0000 | | |
| $a(Å)$ | 4.836900 | | |
| $b(Å)$ | 4.836900 | | |
| $c(Å)$ | 7.885000 | | |
| $RF_2$ | 12.09 | | |
| $RF_2w$ | 15.03 | | |
| $RF$ | 6.351 | | |
| $\chi_2$ | 1.924 | | |

imately 5 kHz) along with the wider aperture that we allowed to increase the neutron counts for the magnetic measurements. To determine detector saturation, we fitted the ratios of 4 K amplitudes (measured with analyser, single-counter detctor and wide apterture) to 20 K amplitudes (measured without analyser, with PSD and narrow amplitude) using an exponential function. The resulting refinement is shown in Fig. 10 and Table V. Similar to the nuclear refinement in the paramagnetic state, we find good agreement with corrected intensities.

The lattice parameters were calculated from the centers of the peaks and slightly increased with the reduction in temperature with the appearance of magnetic order, especially in the easy magnetization c axis. The change though is extremely small (0.01% in a,b and 0.1% in c axis to claim the presence of magnetostriction with high confidence).

## REFINEMENT OF THE SDW STRUCTURE BASED ON THE $\Gamma_2$ REPRESENTATION

The SDW data at 4 K with peaks at equivalent positions of ordering wave vector $\mathbf{q}_{\mathrm{SDW}}$ =(0 0 0.156) had an average intensity of 19.2 counts after monitor correction. We corrected the intensities for the single-counter-detector influence on the measured peak widths and for saturation as described above. For refining corrected magnetic peaks the same extinction parameter was used as for the nuclear data set at 20 K, although there is no significant effect due to the much smaller scale of magnetic intensities. The comparison of measured vs refined intensities is given in Table VI.

The absolute-moment scale has been obtained by comparing the corrected intensities of nuclear and magnetic peaks at 4K̃. Additionally, similar values have been obtained independent of the single-counter-detector saturation effect by just using weak nuclear peaks. Thirdly, the comparision of nuclear and magnetic peaks measured

| h | k | l | $F^2_{\text{obs}}$ | $\sigma$ | $F^2_{\text{cal}}$ | Dif/$\sigma$ | $\sin\theta/\lambda$ |
|---|---|---|---|---|---|---|---|
| 0 | 0 | 1.844 | 0.0060 | 0.0100 | 0.0000 | 0.6000 | 0.1169 |
| -1 | 0 | -0.156 | 0.4487 | 0.1940 | 0.5856 | -0.7056 | 0.1198 |
| -1 | 0 | 0.844 | 5.7671 | 0.3589 | 6.6615 | -2.4920 | 0.1308 |
| 0 | 0 | 2.156 | 0.0000 | 0.0900 | 0.0000 | -0.0002 | 0.1367 |
| -1 | 0 | -1.156 | 5.4364 | 0.3241 | 6.3395 | -2.7864 | 0.1401 |
| 0 | -1 | -1.844 | 4.0400 | 0.3397 | 4.5648 | -1.5448 | 0.1671 |
| -1 | 0 | 2.156 | 4.5157 | 0.3965 | 3.7990 | 1.8077 | 0.1815 |
| -1 | -1 | -0.156 | 15.6396 | 1.0020 | 15.0400 | 0.5984 | 0.2070 |
| 0 | -1 | -2.844 | 2.3146 | 0.4325 | 2.0643 | 0.5787 | 0.2163 |
| -1 | 0 | -3.156 | 1.7184 | 0.4515 | 1.5272 | 0.4235 | 0.2330 |
| -1 | -1 | -1.844 | 1.3478 | 0.4300 | 1.3962 | -0.1126 | 0.2375 |
| 0 | -2 | 0.156 | 27.2289 | 3.1540 | 24.9411 | 0.7254 | 0.2389 |
| 0 | 0 | 3.844 | 0.0100 | 0.2000 | 0.0000 | 0.0500 | 0.2438 |
| 0 | -2 | 0.844 | 38.3307 | 3.2267 | 36.9193 | 0.4374 | 0.2447 |
| 1 | -2 | 2.156 | 1.2295 | 0.4167 | 1.0523 | 0.4252 | 0.2479 |
| -2 | 0 | 1.156 | 35.1288 | 1.7209 | 33.6652 | 0.8505 | 0.2497 |
| 0 | 0 | 4.156 | 0.1000 | 0.3000 | 0.0000 | 0.3333 | 0.2635 |
| 0 | -2 | -1.844 | 3.2069 | 0.8336 | 3.6070 | -0.4800 | 0.2658 |
| 0 | -1 | -3.844 | 0.9381 | 0.3500 | 0.0174 | 2.6304 | 0.2714 |
| -2 | 0 | 2.156 | 3.2829 | 1.0090 | 3.1502 | 0.1315 | 0.2751 |
| -1 | 0 | 4.156 | 0.7279 | 0.4890 | 0.0251 | 1.4371 | 0.2893 |
| 0 | -2 | -2.844 | 13.6547 | 1.1644 | 15.3913 | -1.4914 | 0.2992 |
| 0 | -2 | 3.156 | 12.6293 | 1.0202 | 12.8420 | -0.2085 | 0.3115 |
| -1 | -2 | 0.156 | 0.0010 | 0.2000 | 0.1030 | -0.5101 | 0.3160 |
| 1 | 1 | 3.844 | 3.3710 | 0.8457 | 3.0213 | 0.4135 | 0.3196 |
| -2 | -1 | 1.156 | 2.3244 | 0.6850 | 1.7265 | 0.8729 | 0.3203 |
| -2 | -1 | -1.156 | 2.1840 | 0.6900 | 1.6470 | 0.7782 | 0.3242 |

TABLE VI. SDW intensities at 4 K and calculated intensities by refinement of the $\Gamma_2$ representation with FullProf.

at WISH with a single setup confirms the obtained scale within the error. The uncertainty of the overall scale factor, which shifts all extracted magnetic moments to higher or lower values simultaneously, is 7%.

## REFINEMENT OF $\Gamma_2$ REPRESENTATION WITH FE MOMENTS ALONG THE $c$ AXIS ONLY

The observed SDW structure has also been modeled with the reduced parameter space of the $\Gamma_2$ representation that limits magnetic moments to Fe sites and their moments to the easy $c$ axis. A comparison of measured Bragg peak intensities and calculated values based on Rietveld refinement is shown in Fig. 11. Associated refined parameters are listed in Table VII.

Refining only $c$ axis amplitudes of the Fe moments still yields good modeling of the measured data and is only slightly worse compared to including Nb moments. Removing $Fe_{2a}$ moments while retaining Nb spins (case not

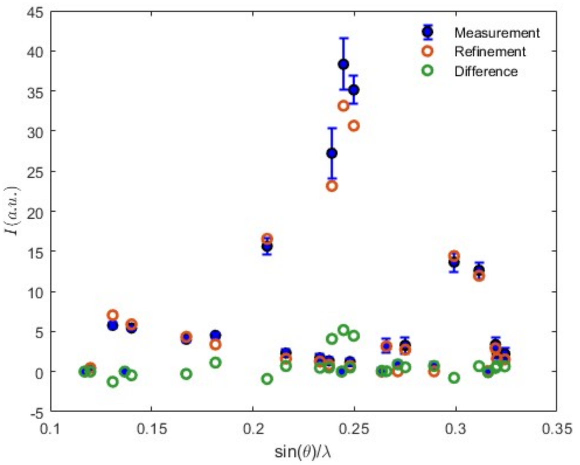


FIG. 11. *SDW structure of $NbFe_2$ at 4 K: measured intensities compared to values calculated from the refinement of the $\Gamma_2$ representation with the constraints of moments being limited to Fe sites and to the c-axis orientation.*

shown here) leads to substantially poorer refinement.

TABLE VII. Refined parameters of the $\Gamma_2$ representation with moments limited to Fe sites and to the $c$ axis to describe the SDW structure at 4 K. $m_{\text{amp}}$ is the amplitude of the net unit-cell magnetic moment. $\bar{m}_{\text{av}}$ is the average magnitude of the net unit-cell magnetic moment. Agreement factors are listed below.

| Site | $S_a$ ($\mu_B$) | $S_b$ ($\mu_B$) | $S_c$ ($\mu_B$) |
|---|---|---|---|
| $Fe_{2a}$ | 0 | 0 | $0.0461 \pm 0.0026$ |
| $Fe_{6h}$ | 0 | 0 | $-0.0808 \pm 0.0014$ |
| $Nb_1$ | 0 | 0 | $0.000 \pm 0.000$ |
| $Nb_2$ | 0 | 0 | $0.000 \pm 0.000$ |
| $m_{\text{amp}}$ ($\mu_B$/atom) | $0.0306 \pm 0.001$ | | |
| $\bar{m}_{\text{av}}$ ($\mu_B$/atom) | $0.0204 \pm 0.001$ | | |
| $R_{F^2}$ | 13.81 | | |
| $R_{F^2w}$ | 16.04 | | |
| $R_F$ | 11.51 | | |
| $\chi^2$ | 2.179 | | |

## REFINEMENT OF THE $\Gamma_2$ REPRESENTATION INCLUDING A-B PLANE COMPONENTS

The observed SDW structure has also been modeled with the inclusion of $ab$-plane moment components. A comparison of measured Bragg peak intensities and calculated values based on Rietveld refinement is shown in Fig. 12. Associated refined parameters are listed in Table VIII.

This refinement shows very good agreement between the calculated and observed magnetic intensities, as reflected by the low reliability factors and a reduced chi-

squared value close to unity. This indicates that the experimental uncertainties are well estimated and that the magnetic model provides a robust description of the data. When allowing the moments in the $ab$ plane to refine freely, their values converge to very small amplitudes within uncertainty, indicating that the ordered moments are effectively confined to the $c$ axis. Overall, these results confirm that the unconstrained $\Gamma_2$ representation captures the essential features of the SDW magnetic structure at 4 K.

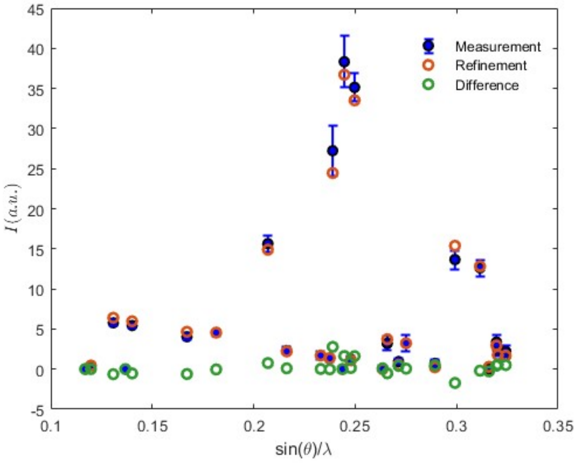


FIG. 12. *SDW structure of* $NbFe_2$ *at 4 K: measured intensities compared to values calculated from the refinement of the* $\Gamma_2$ *representation with the moments having no constraints.*

TABLE VIII. Refined parameters of the $\Gamma_2$ representation with the moments having no constraints to describe the SDW structure at 4 K. $m_{\text{amp}}$ is the amplitude of the net unit-cell magnetic moment. $\bar{m}_{\text{av}}$ is the average magnitude of the net unit-cell magnetic moment. Agreement factors are listed below.

| Site | $S_a$ ($\mu_B$) | $S_b$ ($\mu_B$) | $S_c$ ($\mu_B$) |
|---|---|---|---|
| $Fe_{2a}$ | 0 | 0 | $0.0433 \pm 0.002$ |
| $Fe_{6h}$ | $0.0097 \pm 0.0022$ | 0 | $-0.0855 \pm 0.0012$ |
| $Nb_1$ | 0 | 0 | $-0.0180 \pm 0.0224$ |
| $Nb_2$ | 0 | 0 | $-0.0042 \pm 0.0252$ |
| $m_{\text{amp}}$ ($\mu_B$/atom) | $0.0342 \pm 0.001$ | | |
| $\bar{m}_{\text{av}}$ ($\mu_B$/atom) | $0.0243 \pm 0.001$ | | |
| $R_{F^2}$ | 7.642 | | |
| $R_{F^2w}$ | 9.865 | | |
| $R_F$ | 6.796 | | |
| $\chi^2$ | 0.9365 | | |

## REFINEMENT OF THE $\Gamma_4$ REPRESENTATION

A comparison of measured Bragg peak intensities and calculated values based on Rietveld refinement of the next best irreducible representation $\Gamma_4$, which features antiferromagnetic alignment of symmetrically equivalent sites, is shown in Fig. 13. Associated refined parameters are listed in Table IX.

The refinement is substantially worse compared to the $\Gamma_2$ refinement and adding $a-b$ spin components on the $Fe_{6h}$ does not significantly improve the refinement.

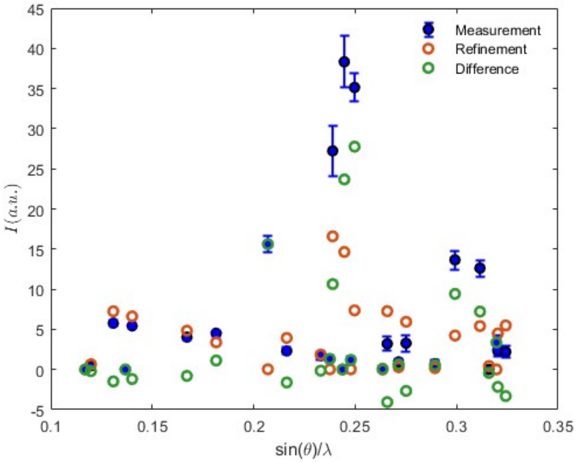


FIG. 13. *SDW structure of* $NbFe_2$ *at 4 K: measured intensities compared to values calculated from the refinement of the* $\Gamma_4$ *representation.*

TABLE IX. Refined parameters of the $\Gamma_4$ representation to describe the SDW structure at 4 K. $m_{\text{amp}}$ is the amplitude of the net unit-cell magnetic moment. $\bar{m}_{\text{av}}$ is the average magnitude of the net unit-cell magnetic moment. Agreement factors are listed below.

| Site | $S_a$ ($\mu_B$) | $S_b$ ($\mu_B$) | $S_c$ ($\mu_B$) |
|---|---|---|---|
| $Fe_{6h,AB}$ | 0 | 0 | $-0.0019 \pm 0.006$ |
| $Fe_{6h,C}$ | 0 | 0 | $-0.0469 \pm 0.011$ |
| $Fe_{2a}$ | 0 | 0 | $0.1042 \pm 0.02$ |
| $Nb_1$ | 0 | 0 | $0.0237 \pm 0.065$ |
| $Nb_2$ | 0 | 0 | $-0.125 \pm 0.033$ |
| $m_{\text{amp}}$ ($\mu_B$/atom) | $0.0418 \pm 0.023$ | | |
| $\bar{m}_{\text{av}}$ ($\mu_B$/atom) | $0.0038 \pm 0.023$ | | |
| $R_{F^2}$ | 65.04 | | |
| $R_{F^2w}$ | 63.36 | | |
| $R_F$ | 43.87 | | |
| $\chi^2$ | 38.63 | | |

[1] Henrik Thoma and Vladimir Hutanu. Snp filescanner-tool for time dependent polarization corrections of polarized diffraction data. In *JCNS Workshop 2018*, number FZJ-2019-00329. Streumethoden, 2018.

[2] M Blume. Polarization effects in the magnetic elastic scat-

tering of slow neutrons. *Physical Review*, 130(5):1670, 1963.

[3] Owen Arnold, Jean-Christophe Bilheux, JM Borreguero, Alex Buts, Stuart I Campbell, L Chapon, Mathieu Doucet, N Draper, R Ferraz Leal, MA Gigg, et al. Mantid—data analysis and visualization package for neutron scattering and $\mu$ sr experiments. *Nuclear instruments and methods in physics research section a: accelerators, spectrometers, detectors and associated equipment*, 764:156–166, 2014.

[4] RB Von Dreele, JD t Jorgensen, and CG Windsor. Rietveld refinement with spallation neutron powder diffraction data. *Journal of Applied Crystallography*, 15(6):581–589, 1982.

[5] PG Niklowitz, M Hirschberger, M Lucas, P Cermak, A Schneidewind, E Faulhaber, J-M Mignot, WJ Duncan, A Neubauer, C Pfleiderer, et al. Ultrasmall moment incommensurate spin density wave order masking a ferromagnetic quantum critical point in nbfe 2. *Physical review letters*, 123(24):247203, 2019.

[6] GJ McIntyre and RFD Stansfield. A general lorentz correction for single-crystal diffractometers. *Acta Crystallographica Section A: Foundations of Crystallography*, 44(3):257–262, 1988.

[7] JH Zhu, LM Pike, CT Liu, and PK Liaw. Point defects in binary laves phase alloys. *Acta materialia*, 47(7):2003–2018, 1999.
